# Supplementary material for: Hierarchically Structured Scheduling and Execution of Tasks in a Multi-Agent Environment
Source: arXiv:2203.03021 source file (2022-03-06)
Supplement: Supplementary file 1 [file supplementary.tex]

\newpage
\appendix
\onecolumn
\section{Supplementary Material}
